# Supplementary material for: Finding Cut-Offs in Leaderless Rendez-Vous Protocols is Easy
Source: arXiv:2010.09471 source file (2023-10-11)
Supplement: Supplementary file 1 [file appendix.tex]

\section*{APPENDIX}

In the following, we will use the notations $M \reachN{\sigma}$
and $\reachN{\sigma} M$ to denote the fact that there exists
$M', M''$ such that $M \reachN{\sigma} M'$ and $M'' \reachN{\sigma} M$
respectively. Similar notation holds for $\reachQ{}$ as well. 

\section{Proofs of Section \ref{sec:lemmas}}
We prove Lemmas \ref{lem:fh} and \ref{lem:fhshort}. Let us first give an intuitive idea of the proof.
Assume $M \reachQ{\sigma} M'$. For the purpose of studying this firing sequence, we can remove from the 
net all transitions that do not occur in $\sigma$, and all places that are neither input nor output places of some transition 
of $\sigma$. Let $\net'$ be the resulting net. We show that $nM \reachQ{\sigma} nM'$ for a sufficiently large $n$.
In a first step, we show in Lemma \ref{lem:saturation} that for a sufficiently large $n$ we can find markings $M_1$ and $M_2$ 
that mark every place of $\net'$ and satisfy the following properties: $nM \reachN{*} M_1$, $M_2 \reachN{*} nM'$.
This reduces the problem to showing that 
that $nM_1 \reachN{} nM_2$ holds for sufficiently large $n$. For this we apply a folklore lemma showing that 
if $L_2 = L_1 + \incidence (m \bx)$ for some number $m$ and some $\bx \in \nn^T$, and
$L_1 \reachN{\tau}$ and $\reachN{\tau} L_2$ for some firing sequence $\tau$ such that $\parikh{\tau} = \bx$, then
$L_1 \reachN{\tau^m} L_2$ where $\tau^m$ denotes the concatentation of 
$\tau$ with itself $m$ times (Lemma \ref{lem:iter}). Finally, we show in Lemma \ref{lem:fh} itself that $M_1$ and $M_2$ can be chosen so that 
for sufficiently large $n$ the markings $L_1:= n M_1$ and $L_2 := n M_2$ satisfy these properties.

\begin{lemma}\label{lem:saturation}
	Let $M$ be a marking such that $M \reachQ{\sigma}$ for
	some firing sequence $\sigma$. Let $m$ be the size of $\supp{\sigma}$
	and let $\weight$ be the weight of $\net$. %and let 
	%$W =  \max \{\|Pre[p,t]\| \mid t \in \supp{\sigma}, p \in \preset{t} \}$.
	There exists a firing sequence  $$\left( (\weight +1)^m \cdot M \right) \xrightarrow{\tau} L$$
	\noindent such that $\supp{\tau} = \supp{\sigma}$, $|\tau| \leq 2 (\weight +1)^m$ and $L(p) > 0$ 
	for every $p \in \supp{M} \cup \pre{\supp{\sigma}} \cup \post{\supp{\sigma}}$
\end{lemma}

\begin{proof}
	Let $t_1, t_2, \ldots, t_m$ be the transitions of $\supp{\sigma}$, sorted according to the order of
	their first occurrence in $\sigma$.   Let $\beta_0 = 1$, $\beta_i = (\weight+1)^{i}$ for every $i \in \{1, \ldots, m\}$, and define the sequence 
	$$\tau_0 = \epsilon$$
	$$\tau_i = t_1^{\beta_{i-1}} t_{2}^{\beta_{i-2}} \cdots t_i^{\beta_0} \ $$
	By the definition of $\beta_i$ we have $|\tau_i| \leq 2 (\weight +1)^i$. We prove for every $i \geq 0$ that 
	$$(\beta_i \cdot M) \xrightarrow{\tau_i} M_i$$
	\noindent for some marking $M_i$ such that $M_i(p) > 0$
	for every $p \in \supp{M} \cup \pre{\supp{\tau_i}} \cup \post{\supp{\tau_i}}$.
	Since $\supp{\tau_m} = \supp{\sigma}$, the lemma then follows by taking $L:=M_m$.
	The proof is by induction on $i$.
	
	\medskip\noindent\textbf{Basis: $i=0$.} Then $\beta_i = 1$ and the result follows from $M \xrightarrow{\epsilon} M$.
	
	%\medskip\noindent\textbf{Basis: $m=1$.} Then $\sigma$ only contains $t_1$. Since $M_0$ enables $\sigma$, it enables $t_1$. Since $\beta(1) = \alpha + 1$ and $t_1$ takes at most $\alpha$ tokens from each of its input places, we have
	%
	%$$(\beta(1) \cdot M_0)  \reachN{t_1} M_1$$
	%
	%\noindent where the marking $M_1$ marks every place marked at $M_0$ and all input and output places of $t_1$. 
	
	\medskip\noindent\textbf{Induction Step:  $i \geq 1$.} Since $M$ enables $\sigma$, it also enables some 
	prefix of $\sigma$ with support $t_1, \ldots, t_{i-1}$. By induction hypothesis,
	$$(\beta_{i-1} \cdot M) \xrightarrow{\tau_{i-1}} M_{i-1}$$
	\noindent  where $M_{i-1}(p) > 0$ for every $p \in \supp{M} \cup \pre{\supp{\tau_{i-1}}} \cup \post{\supp{\tau_{i-1}}}$ . Since $\beta_i = (\weight +1) \beta_{i-1}$ we have
	$$(\beta_i \cdot M)  \xrightarrow{\tau_{i-1}^{(\weight+1)}} \; ((\weight +1) \cdot M_{i-1})$$
	
	\noindent Since  $M \reachQ{\sigma}$ and $t_i$ appears in $\sigma$,
	it follows that every place $p \in \pre{t_i}$
	%So every place in $\pre{t_i}$ 
        has at least $(\weight + 1)$ tokens at the marking $(\weight+1) \cdot M_{i-1}$. So $(\weight+1) \cdot M_{i-1} \xrightarrow{t_i} M_i$ for some marking $M_i$ 
	such that $M_i(p) > 0$ for every $p \in \supp{M} \cup 
	\pre{\{t_1,\dots,t_i\}} \cup \post{\{t_1,\dots,t_i\}}$.
\end{proof}

\begin{lemma}\label{lem:iter}
	Let $(\net, M, M')$ be a Petri net system, and let $\sigma$ be a firing sequence such that $M \xrightarrow{\sigma}$,
	$\xrightarrow{\sigma} M'$, and $n \parikh{\sigma}$ is a solution of the marking equation for some $n \ge 1$.
	Then $M \xrightarrow{\sigma^n} M'$.
\end{lemma}
\begin{proof}
Since $n \parikh{\sigma}$ is a solution of the marking equation, $M \xrightarrow{\sigma^n}$ implies $M \xrightarrow{\sigma^n} M'$. 
So it suffices to prove $M \xrightarrow{\sigma^n}$. We proceed by 
induction on $n$. If $n\leq 2$  then $M \xrightarrow{\sigma^n}$ follows immediately from  $M \xrightarrow{\sigma}$ and $\xrightarrow{\sigma} M'$. Assume $n > 2$, and let $M_1, M_1'$ be the markings such that $M \reachN{\sigma} M_1$ 
and $M_1'  \reachN{\sigma} M'$.

\medskip\noindent We first claim that $M_1 \reachN{\sigma}$ holds.  Let $\sigma = t_1 t_2 \dots t_m$, and let $L_{1}, \dots, L_{m-1}, L_{1}', 
\ldots, L_{m-1}'$ be the markings given by
$$
M  \reachN{t_1}  L_{1} \cdots L_{m-1} \reachN{t_m}  M_1   \qquad \text{ and } \qquad M'_1  \reachN{t_1} L_{1}' \cdots L_{m-1}' \reachN{t_m}  M' \;\; .
$$
Further, let $\sigma_0 := \epsilon$ and $\sigma_i := t_1 \cdots t_i$ for every $1 \leq i \leq m$, and define $K_{i}: = M_1 + \incidence \cdot \parikh{\sigma_i}$.
We prove that $K_{i} \reachN{t_{i+1}}$ holds for every $1 \leq i \leq m$, which implies the claim. It suffices to show that $K_{i}(p) \geq \Pre[p, t_{i+1}]$ holds for every place $p$. Since $L_{i} \reachN{t_{i+1}}$ and $L_{i}' \reachN{t_{i+1}}$, we have $L_{i}(p) \geq \Pre[p, t_{i+1}]$ and 
$L_{i}'(p) \geq \Pre[p, t_{i+1}]$. Let $\sigma[i]$ be the cyclic permutation of $\sigma$ starting at $t_i$. By the definition of $K_i$ we have $K_i = L_i + \incidence \cdot \parikh{\sigma[i]}$.  Since $\incidence \cdot \parikh{\sigma} = \incidence \cdot \parikh{\sigma[i]}$, letting $\Delta := \incidence \cdot \parikh{\sigma}$, we obtain altogether
$$\begin{array}{rclcl}
L_i(p)  &  & & \geq &  \Pre[p, t_{i+1}] \\[0.2cm]
K_i(p) & = & L_i(p) + \Delta(p) &  \\[0.2cm]
L_{i}' (p) & =  & L_{i}(p) + (n-1) \Delta(p) & \geq & \Pre[p, t_{i+1}] 
\end{array}$$
This implies  $K_i(p) \geq \Pre[p,t_{i+1}]$, and the claim is proved. By the claim we have  $M_1 \reachN{\sigma}$; moreover $\xrightarrow{\sigma} M'$, and
$(n-1) \parikh{\sigma}$ is a solution of the marking equation for $(\net,M_1,M')$. By induction hypothesis $M_1 \reachN{\sigma^{n-1}} M'$,
and so $M \xrightarrow{\sigma^n} M'$.
\end{proof}

%\begin{lemma}
%\label{lem:iter}
%Let $(N, M_0)$ be a Petri net. If $M_0 \reachN{\sigma}$, $\reachN{\sigma} M$, and $M = M_0 + \inc{N} \cdot n \cdot \vec{\sigma}$ for some $n \geq 0$, then $M_0 \reachN{\sigma^n} M$.
%\end{lemma}
%\begin{proof}
%TBD.
%\end{proof}

\begin{proposition}\label{prop:easy}
Let $\weight$ be the weight of the net $\net$.
Suppose $M$ is a marking and $\sigma$ is a firing sequence
such that $M(p) \ge \weight \cdot \parikh{\sigma}(t)$ for every $t \in \supp{\sigma}$ and for every $p \in \pre{t}$. Then $M \xrightarrow{\sigma}$.
\end{proposition}

\begin{proof}
Very easy induction on $\sum_{t \in T} \parikh{\sigma}(t)$.
\end{proof}

We are now ready to prove Lemma \ref{lem:fh}.

\ScalingLemmaInFull*
%\begin{lemma}
%\label{lem:fh}
%Let $M_0$ and $M$ be discrete markings such that $M_0 \reachQ{\sigma} M$
%for some firing sequence $\sigma$.
%Let $m$ be the size of $\supp{\sigma}$, $\beta = (W+1)^m$, let
%$k$ be the smallest natural number such that $k \cdot \parikh{\sigma} \in \nn^T$, and let $\ell$ be $\|\parikh{\sigma}\|$. Then, there exists a sequence $\tau$ 
%such that $\supp{\tau} = \supp{\sigma}$ and
%%$|\tau| \leq 4 Wk \ell + 16 W k^2  \ell^2$ and
%$$\left( 16 W \beta^{2} k \ell \cdot M_0 \right) \xrightarrow{\tau} \left( 16 W \beta^{2} k \ell \cdot M \right)$$
%\end{lemma}

\begin{proof}
%First, we note that since $M_0 \reachQ{\sigma} M$ we have
%\begin{equation}\label{eq:marking-Q}
%	M = M_0 + \incidence{\parikh{\sigma}}
%\end{equation}

Let $\beta:= (\weight+1)^m$ and  $\gamma := 4\weight \beta k \ell$.
We split the proof into three parts, by providing the desired firing sequence
as a concatenation of three firing sequences of the form
\begin{equation}~\label{eq:three-parts}
	\left( 4k\beta \gamma \cdot M \right) \xrightarrow{*} 
	\gamma L_1 \xrightarrow{*} \gamma L_2 \xrightarrow{*}
	\left( 4k \beta \gamma \cdot M'\right)
\end{equation}
for some markings $L_1$ and $L_2$.

\subsubsection{First firing sequence: }
Since $M \reachQ{\sigma} M'$, 
by Lemma~\ref{lem:saturation} there exists a firing sequence $\tau_1$ and a marking $M_1$ such that $|\tau_1| \le 2\beta$, 
$\supp{\tau_1} = \supp{\sigma}$, $M_1(p) > 0$ for all $p \in \pre{\supp{\sigma}} \cup \post{\supp{\sigma}}$ and $(\beta \cdot M_0) \xrightarrow{\tau_1} M_1$. Let $L_1 = (4k-1)\beta M + M_1$. It is then clear that
$4k\beta M \xrightarrow{\tau_1} L_1$. From this it is once
again clear that $4k\beta \gamma M \xrightarrow{\tau_1^{\gamma}} \gamma L_1$, thereby completing the first part of the run.
We note that by construction of $L_1$, we have $(\gamma L_1)(p) \ge \gamma$ 
for every $p \in \pre{\supp{\sigma}} \cup \post{\supp{\sigma}}$.

\subsubsection{Third firing sequence: }
The third part is similar to the first part, except that we apply
Lemma~\ref{lem:saturation} to the reverse net. 
Notice that since $\reachQ{\sigma} M'$ in the Petri net $\net$,
it follows that $M' \reachQ{\sigma^{-1}}$ in the \emph{reverse net} $\net^{-1}$ where $\net^{-1} := (P,T,\Post,\Pre)$
and $\sigma^{-1}$ is the reverse of $\sigma$. 
Using Lemma~\ref{lem:saturation}, we can get a firing sequence $\tau_2'$ and a marking $M_2$ such that $|\tau_2'| \le 2\beta$, 
$\supp{\tau_2'} = \supp{\sigma}$, $M_2(p) > 0$ for all $p \in \pre{\supp{\sigma}} \cup \post{\supp{\sigma}}$ and $(\beta \cdot M') \xrightarrow{\tau_2'} M_2$
in the reverse net $\net^{-1}$. Let $L_2 = (4k-1)\beta M' + M_2$.
By the same argument as the first part, we can conclude 
that $4k\beta \gamma M' \xrightarrow{\tau_2'^{\gamma}} \gamma L_2$
in the reverse net $\net^{-1}$.
Letting $\tau_2 := \tau_2'^{-1}$ we get that
$\gamma L_2 \xrightarrow{\tau_2^{\gamma}} 4k\beta \gamma M'$.
We note that by construction of $L_2$, we have $(\gamma L_2)(p) \ge \gamma$ 
for every $p \in \pre{\supp{\sigma}} \cup \post{\supp{\sigma}}$.

\subsubsection{Second firing sequence: }
By construction of $\tau_1$ and $\tau_2$ we have that
$|\tau_1|, |\tau_2| \le 2\beta$. It follows then that
$\|\parikh{\tau_1}\| + \|\parikh{\tau_2}\| \le 4\beta$. Once again by construction
of $\tau_1$ and $\tau_2$ we have that $\supp{\tau_1} = \supp{\tau_2} = \supp{\sigma}$. Further by construction of the number $k$,
it follows that all the non-zero components of $4k\beta \parikh{\sigma}$
are at least $4\beta$. Hence, if we define 
\begin{equation}
\label{eq:fh1.5}
v := 4 \beta k \parikh{\sigma} - (\parikh{\tau}_1 + \parikh{\tau}_2) 
\end{equation}
then $v$ is a non-negative integer vector.

Let $\tau_3$ be any firing sequence such that $\parikh{\tau_3} = v$.
We claim that $\gamma L_1 \xrightarrow{\tau_3}, \xrightarrow{\tau_3} \gamma L_2$
and $\gamma L_2 = \gamma L_1 + \incidence \cdot (\gamma \cdot v)$. Notice that if this claim
is true, then by Lemma~\ref{lem:iter} we have that
$\gamma L_1 \xrightarrow{\tau_3^{\gamma}} \gamma L_2$ and then
the second part of equation~\ref{eq:three-parts} will also be done,
thereby making the proof complete.

All that is left to prove are the three claims. 
As remarked at the end of the first part of the construction,
notice that $(\gamma  L_1)(p) \ge \gamma$ for every $p \in \pre{\supp{\sigma}} \cup \post{\supp{\sigma}}$. Since $\parikh{\tau_3} = v$, 
by equation~\ref{eq:fh1.5} notice
that $\supp{\tau_3} \subseteq \supp{\sigma}$
and $\weight \cdot \|\parikh{\tau_3}\| \le \weight \cdot 4\beta k \cdot \|\parikh{\sigma}\| = \weight \cdot 4\beta k \ell = \gamma$.
Hence it follows that $(\gamma L_1)(p) \ge \weight \|\parikh{\tau_3}\|$ for every $p \in \pre{\supp{\tau_3}} \cup \post{\supp{\tau_3}}$.
Applying proposition~\ref{prop:easy}, we get that $\gamma L_1 \xrightarrow{\tau_1}$.

By the same argument applied to the reverse net $\net^{-1}$,
we can get that $\gamma L_2 \xrightarrow{\tau_2^{-1}}$
in the reverse net $\net^{-1}$, hence leading to 
$\xrightarrow{\tau_2} \gamma L_2$.

Finally, notice that 
$$\begin{array}{lclrr}
L_2 & = & 4 k \beta \cdot  M' - \incidence \cdot \parikh{\tau_2} & \ \qquad \ & \mbox{($L_2 \xrightarrow{\tau_2} 4k\beta \cdot M'$)}\\
& = & 4 \beta k \cdot  M + \incidence \cdot 4 \beta k \cdot \parikh{\sigma}  - \incidence  \cdot \parikh{\tau_2} &  & \mbox{($M \reachQ{\sigma} M'$)}\\
& = & L_1 - \incidence \cdot \parikh{\tau_1} + \incidence \cdot 4 \beta k \cdot \parikh{\sigma} - \incidence \cdot \parikh{\tau_2}  & & \mbox{($4k\beta \cdot M \xrightarrow{\tau_1} L_1$)}\\
& = &  L_1 + \incidence \cdot (4 \beta k \cdot \parikh{\sigma} - (\parikh{\tau_1} + \parikh{\tau_2})) \\
& = & L_1 + \incidence \cdot v & & \mbox{(Equation~\ref{eq:fh1.5})}\\
\end{array}$$
and so $\gamma \cdot L_2 = \gamma \cdot L_1 + \incidence \cdot (\gamma \cdot v)$. Since all the three claims have been proven, the proof is now complete and we have established the desired run.

\end{proof}

Finally, we get the proof of the scaling lemma.

\ScalingLemmaShort*
%\begin{lemma}[Scaling lemma]~\label{lem:scaling-lemma}
%	Suppose $M$ and $M'$ are discrete markings of $\net$ such that
%	$M \xrightarrow[\qnz]{*} M'$. Then 
%        there exists $n \in 2^{O(|\net|)}$ such that 
%	$nM \xrightarrow{*} nM'$.
%\end{lemma}
\begin{proof}
		Suppose $M \xrightarrow[\qn]{*} M'$ for some $\sigma'$.
		By~(\cite{BFHH17}, Proposition 3.2), there is a formula $\phi(M,M',\vect)$ in the existential
		theory of linear rational arithmetic whose size is linear in the size of the net $\net$ such that $\phi(M,M',\bx)$
		is true iff there exists $\sigma$ such that $\parikh{\sigma} = \bx$
		and $M \xrightarrow[\qn]{\sigma} M'$.
		By~(\cite{Sontag85}, Lemma 3.2) if an formula in existential theory of
		linear rational arithmetic is satisfiable, then it 
		is satisfiable by a solution which can be described using 
		a polynomial number of bits in the size of the formula.
		Hence, if there is a solution to $\phi(M,M',\vect)$,
		then there is a solution which can be described using a polynomial
		number of bits in $|\net|(\log \norm{M} + \log \norm{M'})$.
		Combining all this, we get that there is a $\sigma$
		such that the numerator and denominator of every entry of $\parikh{\sigma}$ can be described using
		$(|\net|(\log \norm{M} + \log \norm{M'}))^{O(1)}$ bits and $M \xrightarrow[\qn]{\sigma} M'$.
		
		Notice that the smallest natural number $k$ such that
		$k \cdot \parikh{\sigma} \in \nn^T$ is at most the
		least common multiple of the denominators of all
		the numbers in the vector $\parikh{\sigma}$.
		Since the size of $\supp{\sigma}$ is at most the number of transitions
		of $\net$, if we let $\weight$ be the weight of the net $\net$, then it 
		is easy to verify that the quantities $(\weight+1)^{\supp{\sigma}}$, $\norm{\parikh{\sigma}}$ and $k$
		can all be described using $(|\net|(\log \norm{M} + \log \norm{M'}))^{O(1)}$ bits.
		
		%Since $\norm{\parikh{\sigma}}$ is bounded by $2^{|\net|^{O(1)}}$,
		%it follows then that $k$ and $\|\parikh{\sigma}\|$ are bounded by 
		%$2^{|\net|^{O(1)}}$ as well.

		Applying Lemma~\ref{lem:fh} we now get that there exists
		$n$ with a polynomial number of bits in $|\net|(\log \norm{M} + \log \norm{M'})$ such that $nM \xrightarrow{*} nM'$.
\end{proof}

\section{Proofs of section~\ref{sec:general}}

\FracaHaddard

\begin{proof}
	If $\sigma = \alpha_1 r_1,\dots, \alpha_l r_l$ is a rational firing sequence, let $\sigma/k$ denote the rational firing sequence
	$(\alpha_1/k) r_1,\dots, (\alpha_l/k) r_l$.
	
	Suppose $M \reachQ{\sigma} M'$
	and $M \reachQ{\sigma'} M'$. %where $\sigma = \alpha_1 r_1,\dots,\alpha_k r_k$ and $\sigma' = \beta_1 t_1,\dots,\beta_l t_l$.
	Then notice that $M \reachQ{(\sigma/2) (\sigma'/2)} M'$.
	Consequently the first claim follows.
	
	To prove the second claim, we will use 
	the fact that reachability in continuous Petri nets
	can be decided in polynomial time (\cite{FracaH15}, Proposition 27).
	Let $T = \{t_1,\dots,t_k\}$ be the set of transitions in the net $\net$.
	For each transition $t_i$, we construct a net $\net_{t_i}$ 
	obtained by removing the transition $t_i$ from $\net$.
	We then check if $M'$ can be reached from $M$ over the
	continuous semantics in the net $\net_{t_i}$. By (\cite{FracaH15}, Proposition 27), this can be done in polynomial time.
	Let $\net_{t_{i_1}},\dots,\net_{t_{i_n}}$ be the nets
	for which this is possible, i.e., there exists
	sequences $\sigma_{i_1},\dots,\sigma_{i_n}$
	such that $M'$ can be reached from $M$ by firing 
	$\sigma_{i_j}$ in the net $\net_{t_{i_j}}$.
	It is then clear that $M'$ can be reached from $M$
	in the original net $\net$ by firing the sequence
	$(\sigma_{i_1}/n) (\sigma_{i_2}/n) \dots (\sigma_{i_n}/n)$.
	Hence, it follows that $\{t_{i_1},\dots,t_{i_n}\}$ 
	is the support of the firing sequence with maximum
	support between $M$ and $M'$.

	%We solve $k$ convex semi-linear Horn formulas  $L_1,\dots,L_k$ such that $L_i$ is the following formula:
	%$\exists \bz \ \phi(M,M',\bz) \ \land \ \bz_{t_i} > 0$.
	%Let $L_{i_1},L_{i_2},\dots,L_{i_n}$ be the linear programs
	%which are satisfiable with solutions $\mathbf{u}_{i_1},\dots,\mathbf{u}_{i_n}$ (By Lemma~\ref{lem:poly-time-semi-linear} the satisfiability
	%of each formula can be checked in polynomial time.)
	%It is then clear that
	%$(\sum_{1 \le j \le n} \mathbf{u}_{i_j})/n$
	%is a solution with maximum support for the formula
	%$\exists \bz \ \phi(M,M',\bz)$ and hence 
	%consequently $\{t_{i_1},t_{i_2},\dots,t_{i_n}\}$
	%is the support of the firing sequence with maximum
	%support between $M$ and $M'$.
	
\end{proof}

\Phardness*
\begin{proof}
	We give a logspace reduction from the Circuit Value Problem (CVP)
	which is known to be P-hard~\cite{CVP}.
	
	CVP is defined as follows: Given a boolean circuit $C$ with $n$ 
	input variables $x_1,\dots,x_n$, $m$ gates $g_1,\dots,g_m$, a truth assignment
	$\mathit{v}$ for the input variables and a gate $out$, check if 
	the output is 1 on the gate $out$ under the assignment $\mathit{v}$
	to the input variables.
	
	We represent each gate $g$ as a tuple $(\circ,s_1,s_2)$ where
	$\circ \in \{\lor,\land\}$ denotes the operation of $g$
	and $s_1,s_2 \in \{x_1,\dots,x_n,g_1,\dots,g_m\}$ are the inputs
	to $g$. In a similar fashion each unary gate $g$ is 
	represented as a tuple $(\lnot,s)$. 
	Let $\mathit{v}(x_i) \in \{0,1\}$ denote the 
	assignment of $x_i$ by the valuation $\mathit{v}$.
	
	We now define a rendez-vous protocol as follows:
	Our alphabet $\Sigma$ will be $\{a,b,c\} \cup \{(g,b_1,b_2) : g \text{ is a gate and } b_1,b_2 \in \{0,1\}\}$.
	We will have an initial state $\init$, a final state $\fin$,
	$2n$ states $q_{x_1}^0,q_{x_1}^1,\dots,q_{x_n}^0,q_{x_n}^1$ and 
	$2m$ states $q_{g_1}^0,q_{g_1}^1,\dots,q_{g_m}^0,q_{g_m}^1$.
	The rules are defined as follows:
	\begin{itemize}
		\setlength \itemsep{1mm}
		\item For each $1 \le i \le n$, we have the rules $(\init,!a,q_{x_i}^{\mathit{v}(x_i)})$,
		$(\init,?a,q_{x_i}^{\mathit{v}(x_i)})$. These
		two rules correspond to setting the value of $x_i$ to $\mathit{v}(x_i)$.
		\item For each binary gate $g = (\circ,s_1,s_2)$ 
		and for each $b_1,b_2 \in \{0,1\}$, we have rules
		$(q_{s_1}^{b_1},!(g,b_1,b_2),q_g^{b_1 \circ b_2}),
		(q_{s_2}^{b_2},?(g,b_1,b_2),q_g^{b_1 \circ b_2})$.
		These rules say that if the output of $s_1$ is $b_1$
		and the output of $s_2$ is $b_2$, then set the output of
		$g$ to $b_1 \circ b_2$.
		\item For each unary gate $g = (\lnot,s)$ and each $b \in \{0,1\}$, we have rules
		$(q_s^b,!(g,b),q_g^{\lnot b})$, $(q_s^b,?(g,b),q_g^{\lnot b})$.
		These rules guarantee that the output of $g$ is the negation
		of the output of $s$.
		\item We then have the rules $(q_{out}^1,!b,\fin),(q_{out}^1,?b,\fin)$.
		These rules guarantee that if the output of $out$ is 1,
		then $\fin$ can be reached.
		\item Finally, we have $(\fin,!c,\fin)$ and $(q,?c,\fin)$ for 
		every state $q$. These rules guarantee that once a process
		reaches the state $\fin$, it can make all the other
		processes reach $\fin$ as well.
	\end{itemize}

	It is now clear that the given protocol admits a cut-off
	iff the output of the gate $out$ is 1.
\end{proof}

\section{Proofs of section~\ref{sec:symmetric}}

\SymmOddCase*

\begin{proof}
	$(\Rightarrow)$: Suppose there exists $2k+1 \in \nn$
	and a firing sequence $\sigma$ such that
	$C_{\init}^{2k+1} \xrightarrow{\sigma} C_{\fin}^{2k+1}$. By the marking
	equation it follows that $C_{\fin}^{2k+1} = C_{\init}^{2k+1} + \incidence \parikh{\sigma}$. Taking modulo 2 on both sides of the
	equation, it can be easily seen $\parikh{\sigma} \mod 2$
	is a solution to the system $Eq$ over the $\mathbb{F}_2$.\\
	
	$(\Leftarrow)$: Suppose $Eq$ has a solution $\bx$ over $\mathbb{F}_2$. Let $T'$ be the set of all transitions $t$ such that $\bx[t] = 1$. Let $n = 2|Q|+3$ and consider the configuration $C_{\init}^n$.
	We now construct a run from $C_{\init}^n$ to $C_{\fin}^n$ as follows:
	
	\paragraph*{\textbf{First stage - Saturate: }} 
	Let $G \subseteq Q$ be the set of good states and
	let $l = 2|Q| - 2|G|$.
	By proposition~\ref{prop:impor}, from the configuration $C_{\init}^n$
	we can reach the configuration $\mathtt{First} := \multiset{(2l+3) \cdot \init} + \sum_{q \in G} \multiset{2q}$. This completes the first stage.
	
	\paragraph*{\textbf{Second stage - Insert: }} 
	Notice that every transition $t \in T'$ is enabled 
	at the configuration $\mathtt{First}$. Hence,
	we can fire all these transitions exactly once, in any order,
	from the configuration $\mathtt{First}$ to reach some
	configuration $\mathtt{Second}$. It is easy
	to see that $\mathtt{Second}(q) = 0$ for any bad state $q$.
	We claim that
	$\mathtt{Second}(q) \equiv 0 \mod 2$ for every $q \neq \fin$
	and $\mathtt{Second}(q_f) \equiv 1 \mod 2$.
	Indeed, notice that for every $q \notin \{\init,\fin\}$,
	by the marking equation $\mathtt{Second}(q)-\mathtt{First}(q) = \sum_{t \in T} \incidence[q,t] \cdot \bx[t]$. Since
	$\bx$ is a solution to $Eq$, it follows that
	$\sum_{t \in T} \incidence[q,t] \cdot \bx[t] \equiv 0 \mod 2$, and so we can conclude that
	the difference $\mathtt{Second}(q)-\mathtt{First}(q)$ is even.
	Since $\mathtt{First}(q)$ is even, it follows that
	so is $\mathtt{Second}(q)$. 
	Similarly we can argue that $\mathtt{Second}(\init)$ is even
	and $\mathtt{Second}(\fin)$ is odd. This completes the second stage.
	
	\paragraph*{\textbf{Third stage - Desaturate: }} Notice that
	$\mathtt{Second}(q) = 0$ for any bad state $q$ and
	$\mathtt{Second}(q)$ is even for every $q \neq \fin$.
	By proposition~\ref{prop:impor} it follows that
	from $\mathtt{Second}(q)$ we can reach the configuration
	$C_{\fin}^{n}$, thereby constructing the required run.
\end{proof}

\section{Proofs of section~\ref{sec:symmetric-leader}}

Since $(q,!a,q') \in R$ iff $(q,?a,q') \in R$ for a symmetric protocol,
in the sequel, we will simply denote rules of a symmetric protocol as a tuple in $Q \times \Sigma \times Q$, with the understanding that
$(q,a,q')$ denotes that there are two rules
of the form $(q,!a,q')$ and $(q,?a,q')$ in the protocol. 

Let $\prot$ be a fixed symmetric leader protocol. We recall from the construction of the net $\net_{\prot}$
that the weight of $\net_{\prot}$ is 2, i.e., the largest absolute value 
appearing in the $\Pre$ and $\Post$ matrices of $\net_{\prot}$ is 2.

\Compatibility

\begin{proof}
	Let $n = \|\bx\|$. We will construct a series of 
	compatible pairs $(C_0,\bx_0),(C_1,\bx_1)$,
	$\dots,(C_n,\bx_n)$ 
	and a series of transitions $t_1,\dots,t_n$ such that
	\begin{itemize}
		\item $C_0 = C, \ \bx_0 = \bx$
		\item $C_i \xrightarrow{t_{i+1}} C_{i+1}$ for every $i < n$.
		\item $\bx_{i+1} = \bx_i[\cmm{t_{i+1}}]$ for every $i < n$.
		\item $C_i(q) \ge 2n - 2i$ for every $q \in Q^F$ and every $i < n$.
	\end{itemize}
	
	Suppose we have already constructed the pair $(C_i,\bx_i)$ for 
	some $i < n$. We consider three cases:
	
	\paragraph*{\textbf{Case 1: }} $\bx_i[t] > 0$ for some follower-only transition $t$:
	By assumption $C_i(q) \ge 2n- 2i \ge 2$ for every $q \in Q^F$.
	Hence, it follows that the transition $t$ can be fired at $C_i$. We let $t_{i+1} := t$, $C_i \xrightarrow{t} C_{i+1}$ and let $\bx_{i+1} = \bx_{i}[\cmm{t}]$. 
	It can be easily checked that $(C_{i+1},\bx_{i+1})$ is a compatible pair.
	
	\paragraph*{\textbf{Case 2: }} Suppose $\bx_i[t] > 0$ for some leader transition $t$. Therefore the graph $\gr(\bx_i)$ is not empty. Let $p = lead(C_i)$. We split this into two cases:
	
	\paragraph*{\textbf{Case 2a): }} $p$ is part of some cycle in $\gr(\bx_i)$:
	Let $p,r_1,p_1,r_2,p_2,\dots,p_k,r_{k+1},p$ be a cycle 
	in $\gr(\bx)$. By construction of $\gr(\bx)$, each $r_i$ is a leader transition and $\bx[r_i] > 0$. 
	Since $p = lead(C_i)$ it follows that $C_i(p) > 0$.
	Further, by assumption 
	$C_i(q) \ge 2n - 2i \ge 2$ for every $q \in Q^F$.
	It follows then that $r_1$ is a transition
	which can be fired at the configuration $C_i$. 
	We let $t_{i+1} := r_1$, $C_i \xrightarrow{r_1} C_{i+1}$
	and $\bx_{i+1} := \bx_i[\cmm{r_1}]$. We now have to argue
	that $(C_{i+1},\bx_{i+1})$ is compatible and $C_{i+1}(q) \ge 2n - 2(i+1)$ for every $q \in Q^F$.
	
	Since it is easy to see that $C_{i+1} + \incidence \bx_{i+1} = C_i + \incidence \bx_i$,
	it follows from the compatibility of $(C_i,\bx_i)$ that $C_{i+1} + \incidence \bx_{i+1} \ge 0$.
	Further since $C_i(q) \ge 2n - 2i$ for every $q \in Q^F$,
	it follows that $C_{i+1}(q) \ge 2n - 2(i+1)$ as well.
	
	All that is left to prove is that every vertex in $\gr(\bx_{i+1})$ is reachable from $lead(C_{i+1})$ which is $p_1$.
	Let $s$ be any vertex of $\gr(\bx_{i+1})$.
	Notice that the graph $\gr(\bx_{i+1})$ is necessarily a sub-graph of $\gr(\bx_i)$.
	By compatibility of $(C_i,\bx_i)$, it follows
	that $s$ is reachable from $p$ in $\gr(\bx_i)$.
	Let $p,tr_1,s_1,tr_2,s_2,\dots,s_l,tr_{l+1},s$ be a
	path in $\gr(\bx_i)$. If $tr_1 = r_1$ then $s_1 = p_1$
	and hence $p_1,tr_2,s_2,\dots,s_l,tr_{l+1},s$
	is a path in $\gr(\bx_{i+1})$.
	If $tr_1 \neq r_1$ then $p_1,r_2,p_2,\dots,p_k,r_{k+1},p,tr_1,s_1,\dots,s_l,tr_{l+1},s$
	is a path in $\gr(\bx_{i+1})$. Hence we are done.
	
	\paragraph*{\textbf{Case 2b): }} $p$ is not part of some cycle in $\gr(\bx_i)$:
	Let $Out = \{out_1,\dots,out_b\}$ be the set of leader transitions $t$
	such that $t.\fromstate = p$ and let
	$In = \{in_1,\dots,in_a\}$ be the set of leader transitions
	$t$ such that $t.\tostate = p$. Notice that $Out$ and
	$In$ depend only on $\prot^L$ and \emph{not}
	on $\gr(\bx_i)$.
	
	We claim that for every $in \in In$, $\bx_i[in] = 0$ 
	and there is exactly one $out \in Out$ such that $\bx_i[out] > 0$. 
	Since $(C_i,\bx_i)$ is compatible, every vertex in $\gr(\bx_i)$ is reachable from $p$ and by assumption $p$ is not 
	part of any cycle in $\gr(\bx_i)$. It follows
	then that there are no incoming edges to $p$ in $\gr(\bx_i)$
	and hence $\bx_i[in] = 0$ for every $in \in In$. 
	Once again since every vertex in $\gr(\bx_i)$ is reachable
	from $p$ and since $\gr(\bx_i)$ is not empty, it follows
	that there is at least one $out \in Out$
	such that $\bx_i[out] > 0$. 
	Finally, since $C_i + \incidence\bx_i \ge \textbf{0}$
	it follows that $C_i(p) + \sum_{in \in In} \bx_i[in] - \sum_{out \in Out} \bx_i[out] \ge 0$. Since $\bx_i[in] = 0$ for every $in \in In$ and since $C_i(p) = 1$, it follows that
	there is exactly one $out \in Out$ such that
	$\bx_i[out] > 0$. Hence, by construction of $\gr(\bx_i)$,
	there is exactly one outgoing edge from $p$ in $\gr(\bx_i)$.
	
	Let $r$ be the only outgoing edge in $\gr(\bx_i)$.
	We let $t_{i+1} := r$, $C_i \xrightarrow{r} C_{i+1}$
	and $\bx_{i+1} := \bx_i[\cmm{r}]$. It is once again
	easy to see that $C_{i+1} + \incidence \bx_{i+1} \ge 0$,
	and also that $C_{i+1}(q) \ge 2n - 2(i+1)$ for every $q \in Q^F$.
	
	All that is left to prove is that every vertex in $\gr(\bx_{i+1})$ is reachable from $lead(C_{i+1})$ which is $r.\tostate$.
	Let $s$ be any vertex of $\gr(\bx_{i+1})$.
	Notice that the graph $\gr(\bx_{i+1})$ is necessarily a sub-graph of $\gr(\bx_i)$.
	By compatibility of $(C_i,\bx_i)$, it follows
	that $s$ is reachable from $p$ in $\gr(\bx_i)$.
	Let $p,tr_1,s_1,tr_2,s_2,\dots,s_l,tr_{l+1},s$ be a
	path in $\gr(\bx_i)$. Since $p$ has only one outgoing 
	edge in $\gr(\bx_i)$ (which is $r$), it follows
	that $tr_1 = r$ and $s_1 = r.\tostate$. Hence 
	$s_1,tr_2,s_2,\dots,s_l,tr_{l+1},s$
	is a path in $\gr(\bx_{i+1})$ and so we are done.
	
	Finally it is clear that the constructed 
	sequence $C_0 \xrightarrow{t_1} C_1 \xrightarrow{t_2} \dots 
	\xrightarrow{t_n} C_n$ is the required firing sequence.
\end{proof}

\LeaderCharac

\begin{proof}
		($\Rightarrow$): Suppose there exists $k \in \nn$ such that
		$k \equiv par \ (\text{mod} \ 2)$ and
		a firing sequence $\sigma$ such 
		that $C_{\init}^{k} \xrightarrow{\sigma} C_{\fin}^{k}$. 
		Let $\bx = \parikh{\sigma}$.
		By the marking equation $C_{\fin}^{k} = C_{\init}^{k} + \incidence \bx$. Since $C_{\fin}^k \ge \textbf{0}$, to prove
		that $(C_{\init}^k,\bx)$ is compatible it is enough to
		prove that every vertex in $\gr(\bx)$ is
		reachable from $lead(C_{\init}^k) = \init^L$.
		
		Let $t_1,\dots,t_l$ be leader transitions
		sorted by the order in which they appear in the firing sequence
		$\sigma$. We want to show that for every $i$, the states
		$t_i.\fromstate$ and $t_i.\tostate$ are reachable from $\init^L$
		in $\gr(\bx)$. Notice that for each $t_i$,
		we have that $t_i.\fromstate \in \{\init^L,t_1.\tostate,t_2.\tostate,\dots,t_{i-1}.\tostate\}$.
		Using this and by induction on $l$, we can easily
		prove our claim.

		\medskip \noindent ($\Leftarrow$): Suppose there exists $n \in \nn, \ \bx \in \nn^T$ such that $n \equiv par \ (\text{mod} \ 2)$, $(C_{\init}^n,\bx)$ is compatible and $C_{\fin}^{n} = C_{\init}^{n} + \incidence \bx$.
		We will now find a $k \in \nn$ such that $k \equiv par \ (\text{mod} \ 2)$ and $C_{\init}^{k} \xrightarrow{\sigma} C_{\fin}^{k}$. 
		
		\paragraph*{\textbf{First stage - Saturate: }} In this stage,
		we mark all the places in $Q$ with a lot of tokens by using proposition~\ref{prop:important}. 
		More formally, let $\lambda = 2\|\bx\| \cdot |Q|$ and let $k := \lambda + n$. Note that $k \equiv par \ (\text{mod} \ 2)$.
		By proposition~\ref{prop:important}, from $C_{\init}^{k}$
		we can reach the marking $\mathtt{First} := C_{\init}^{n} + \sum_{q \in Q} \multiset{2\|\bx\| \cdot q}$.
		
		\paragraph*{\textbf{Second stage - Insert: }} 
		Since $(C_{\init}^n,\bx)$ is a compatible pair,
		it follows that $(\mathtt{First},\bx)$ is a compatible pair as well.
		By Lemma~\ref{lem:compatible} it follows that
		there exists a firing sequence $\xi$ such that $\parikh{\xi} = \bx$
		and $\mathtt{First} \xrightarrow{\xi}$.
		By the marking equation, it is clear that, $\mathtt{First} 
		\xrightarrow{\xi} \mathtt{Second}$ where
		$\mathtt{Second} := C_{\fin}^n + \sum_{q \in Q} \multiset{2\|\bx\| \cdot q}$.
		
		\paragraph*{\textbf{Third stage - Desaturate: }} 
		By proposition~\ref{prop:important} from $\mathtt{Second}$
		we can reach the marking $C_{\fin}^n + \multiset{(2\|\bx\| \cdot |Q|) \cdot q_f} = C_{\fin}^k$.
		This concludes the third stage and creates the desired
		run from $C_{\init}^k$ to $C_{\fin}^k$.	
		
\end{proof}

\NPhardness*

\begin{proof}
	We prove NP-hardness by giving a reduction from 3-CNF-SAT.
	Let $\varphi = C_1 \land C_2 \land \dots \land C_m$
	be a 3-CNF formula with variables $x_1,\dots,x_n$,
	where each clause $C_j$ is of the form
	$C_j := \ell_{j_1} \lor \ell_{j_2} \lor \ell_{j_3}$.
	for some literals $\ell_{j_1},\ell_{j_2},\ell_{j_3}$.
	We now construct a symmetric leader protocol as follows:
	
	Our alphabet $\Sigma$ will contain the following symbols:
	For each clause $C_j$, we will have a symbol $c_j$.
	Further, we will also have a special symbol $a$.
	
	The leader's initial state $\init^L$ will be denoted by $p_0$.
	For each variable $x_j$ with $1 \le j \le n$, the leader will have
	three states $p_j, \top_j$ and  $\bot_j$.
	The leader's final state $\fin^L$ will be denoted by $p_n$.
	
	The follower's initial state $\init^F$ will be denoted by $q_0$.
	For each clause $C_j$ with $1 \le j \le m$, the follower will have
	a state $q_j$. The follower's final state $\fin^F$ will be denoted by $q_m$.
	
	For each $0 \le j \le n-1$, the rules for the leader at the
	state $p_j$ are given by the gadget in Figure~\ref{fig:gadget-leader}.
	Intuitively, if the leader decides to move to 
	$\top_{j+1}$ (resp. $\bot_{j+1}$) then she has decided to 
	set the variable $x_{j+1}$ to true (resp. false). 
	Hence, upon moving
	to $\top_{j+1}$ (resp. $\bot_{j+1}$), the leader tries to 
	transmit the clauses which have become true by setting
	$x_{j+1}$ to true (resp. false).

	\begin{figure}[h] 
		\begin{center}
			\tikzstyle{node}=[circle,draw=black,thick,minimum size=5mm,inner sep=0.75mm,font=\normalsize]
			\tikzstyle{edgelabelabove}=[sloped, above, align= center]
			\tikzstyle{edgelabelbelow}=[sloped, below, align= center]
			\begin{tikzpicture}[->,node distance = 1.25cm,scale=0.8, every node/.style={scale=0.8}]
			\node[node] (li) {$p_j$}; 
			\node[node, above right = of li, xshift = 2cm] (ti) {$\top_{j+1}$};
			\node[node, below right = of li, xshift = 2cm] (bi) {$\bot_{j+1}$};
			\node[node, below right = of ti, xshift = 2cm] (H) {$p_{j+1}$}; 
			
			\draw (li) edge[edgelabelabove,] node{$a$} (ti);
			\draw (li) edge[edgelabelbelow,] node{$a$} (bi);
			
			\draw (ti) edge[edgelabelabove] node{$a$} (H);
			\draw (ti) edge[loop above] node{$c_{k_1},c_{k_2},\dots,c_{k_r}$} (ti);
			%\draw (ti) edge[edgelabelbelow] node{$\cpp{D_{q_1}} \land \dots \land \cpp{D_{q_j}}$} (H);
			
			\draw (bi) edge[edgelabelbelow] node{$a$} (H);
			\draw (bi) edge[loop below] node{$c_{l_1},c_{l_2},\dots,c_{l_w}$} (bi);
			%\draw (bi) edge[edgelabelbelow] node{$\cpp{D_{r_1}} \land \dots \land \cpp{D_{r_l}}$} (H);
			
			\end{tikzpicture}
			\caption{Gadget at a state $p_j$. 
				Here $C_{k_1},\dots,C_{k_r}$ denote the set of 
				all clauses in which the literal $x_j$ appears
				and $C_{l_1},\dots,C_{l_w}$ denote the set of all
				clauses in which the literal $\bar{x_j}$ appears.}
			\label{fig:gadget-leader}
		\end{center}
	\end{figure}

	The rules for the followers are very simple:
	For each $0 \le j \le m-1$, there is a rule 
	$(q_j,c_{j+1},q_{j+1})$. Further, there is a special rule $(q_0,a,q_m)$.\\

	We now claim that there is a cut-off for this protocol iff
	the formula $\varphi$ is satisfiable. The first observation 
	we note is the following: From the 
	configuration $\multiset{p_0, 2n \cdot q_0}$ we can
	reach the configuration $\multiset{p_n, 2n \cdot q_m}$.
	Indeed, it is easy to verify that the following is indeed 
	a run in the protocol:
	$\multiset{p_0, 2n\cdot q_0}) \rightarrow \multiset{\top_1, (2n-1)\cdot q_0, q_m}
	\rightarrow \multiset{p_1, (2n-2)\cdot q_0, 2 \cdot q_m}
	\rightarrow \multiset{\top_2, (2n-3)\cdot q_0, 3 \cdot q_m}
	\rightarrow \multiset{p_2, (2n-4)\cdot q_0, 4 \cdot q_m}
	\rightarrow \dots \multiset{\top_{n-1}, q_0, (2n-1) \cdot q_m}
	\rightarrow \multiset{p_n, 2n \cdot q_m}$.  
	
	Since there is always an initial configuration with an even number
	of followers from which we can reach the final configuration,
	by proposition~\ref{prop:even-odd-leader},
	for our reduction to be correct,
	it suffices to prove that there exists $2l+1$ 
	such that there is a run between $\multiset{p_0, (2l+1) \cdot q_0}$ and
	$\multiset{p_n, (2l+1) \cdot q_m}$ iff the formula $\varphi$ is satisfiable.
	
	($\Leftarrow$): Suppose $\varphi$ is satisfiable.
	Let $T$ be a satisfying assignment of $\varphi$ to the variables.
	Let $var(x_j)$ be $\top_j$ if $T(x_j)$ is true
	and let it be $\bot_j$ otherwise. 
	We now construct a run between $\multiset{p_0, (2m+2n+1) \cdot q_0}$
	and $\multiset{p_n, (2m+2n+1) \cdot q_m}$. 
	
	By proposition~\ref{prop:important},
	it is easy to see that from the configuration
	$\multiset{p_0, (2m+2n+1) \cdot q_0}$ we can reach the configuration
	$\mathtt{First} := \multiset{p_0, (2n+1)q_0} + \sum_{1 \le i \le m} \multiset{2q_i}$.
	
	Let $U = \emptyset$.
	From the configuration $\mathtt{First}$, 
	we construct a run which moves the leader from $p_0$ to $p_n$ 
	in the following manner:
	Suppose the leader is currently at $p_j$ for some $j$. 
	We move the leader from $p_j$ to $var(x_{j+1})$ and
	a single follower from $q_0$ to $q_m$ by using the rules
	$(p_j,!a,var(x_{j+1}))$ and $(q_0,?a,q_m)$ respectively.
	Then as long as the leader is at the state $var(x_{j+1})$, 
	we do the following:
	\begin{itemize}
		\item If there is a rule $(var(x_{j+1}),!c_k,var(x_{j+1}))$
		such that $c_k \notin U$, then we keep the
		leader at $var(x_{j+1})$
		and move a single follower from $q_{k-1}$ to $q_{k}$ by using the rules
		$(var(x_{j+1}),!c_k,var(x_{j+1}))$ and $(q_{k-1},?c_{k},q_{k})$. Then, we add the symbol $c_k$ to the set $U$.
		\item If there is no such rule, then 
		we move the leader from $var(x_{j+1})$ to $p_{j+1}$
		and a single follower from $q_0$ to $q_m$ by using the rules
		$(var(x_{j+1}),!a,p_{j+1})$ and $(q_0,?a,q_m)$ respectively.
	\end{itemize}
	
	For every $1 \le k \le m$, notice that the message $c_k$ is 
	sent at most once
	by the leader. Further, since $T$ is a satisfying assignment, 
	it follows that for every $1 \le k \le m$, the message $c_k$ is 
	sent exactly once by the leader.
	Hence, at the end of this procedure, exactly $2n$ followers
	would have moved from $q_0$ to $q_m$ using the rule $(q_0,?a,q_m)$,
	and for every $0 \le k \le m-1$, exactly 1 follower
	would have moved from $q_k$ to $q_{k+1}$.
	It then follows that at the end of this procedure,	
	we would have reached the configuration
	$\mathtt{Second} := \multiset{p_n, (2n+3) q_m} + \sum_{1 \le i \le m-1} \multiset{2q_i}$.
	Once again using proposition~\ref{prop:important},
	from $\mathtt{Second}$ we can reach the configuration
	$\multiset{p_n, (2m+2n+1)q_m}$.
	
	\medskip \noindent
	($\Rightarrow$: ) Suppose there exists $2l+1$ such that there
	is a run between $\multiset{p_0, (2l+1) \cdot q_0}$ and
	$\multiset{p_n, (2l+1) \cdot q_m}$. Notice that along
	the run, for every $1 \le j \le n$, the leader
	has to visit exactly one of $\top_j$ or $\bot_j$.
	This naturally leads us to an assignment $T$
	for the variables as follows: We set $T(x_j)$ to be true
	if the leader visited the state $\top_j$ along the run, 
	otherwise we set $T(x_j)$ to be false.
	
	We now claim that along the run, for every $1 \le j \le m$,
	the leader sent (or) received the message $c_j$. By construction
	of the leader protocol and by construction of the assignment $T$, 
	this would immediately imply
	that $T$ is a satisfying assignment for $\varphi$.
	
	To prove this, first notice that the number of times the leader sends or receives the message
	$a$ in order for her 
	to move from $p_0$ to $p_n$ is exactly $2n$. This implies that the 
	rule $(q_0,a,q_m)$ was used by an even number of followers 
	along the run.
	Since there are $2l+1$ followers to begin with,
	it follows that an odd number of followers had to use the path
	$(q_0,c_1,q_1),(q_1,c_2,q_2),\dots(q_{m-1},c_m,q_m)$ to reach
	the state $q_m$. If the leader had neither sent nor received the message
	$c_j$, then the only way for a follower to move out of
	the $q_{j-1}$ state is to pair with a corresponding follower
	at the state $q_{j-1}$,
	at which point both the followers will go to the state $q_{j}$.
	It then follows that followers could only move out of the
	state $q_{j-1}$ in pairs. However, since an odd number of followers
	reach the state $q_{j-1}$, it would then follow that not all
	the followers could reach the final state $q_m$, which will then
	lead to a contradiction.

\end{proof}
